# Supplementary material for: Invariance-powered Trustworthy Defense via Remove Then Restore
Source: arXiv:2402.00304 source file (2024-02-01)
Supplement: Supplementary file 1 [file X_suppl.tex]

%\clearpage
%\setcounter{page}{1}
%\maketitlesupplementary
%
%
%\section{Rationale}
%\label{sec:rationale}
%%
%Having the supplementary compiled together with the main paper means that:
%%
%\begin{itemize}
%\item The supplementary can back-reference sections of the main paper, for example, we can refer to \cref{sec:intro};
%\item The main paper can forward reference sub-sections within the supplementary explicitly (e.g. referring to a particular experiment);
%\item When submitted to arXiv, the supplementary will already included at the end of the paper.
%\end{itemize}
%%
%To split the supplementary pages from the main paper, you can use \href{https://support.apple.com/en-ca/guide/preview/prvw11793/mac#:~:text=Delete%20a%20page%20from%20a,or%20choose%20Edit%20%3E%20Delete).}{Preview (on macOS)}, \href{https://www.adobe.com/acrobat/how-to/delete-pages-from-pdf.html#:~:text=Choose%20%E2%80%9CTools%E2%80%9D%20%3E%20%E2%80%9COrganize,or%20pages%20from%20the%20file.}{Adobe Acrobat} (on all OSs), as well as \href{https://superuser.com/questions/517986/is-it-possible-to-delete-some-pages-of-a-pdf-document}{command line tools}. 
